# Supplementary material for: Cost-benefit Analysis of Visualization in Virtual Environments
Source: arXiv:1802.09012 ancillary file (2018-02-28)
Supplement: Supplementary file 1 [file CoverLetter.pdf]

Dear EuroVis 2018 co-chairs, IPC members, and Reviewers

**Re: #1065, Cost-benefit Analysis of Visualization in Virtual Environments**

This paper was submitted to SciVis 2017, and was not accepted with scores (3.5, 3, 3, 2). We have provided our feedback at the end of this letter, which is then followed by the original SciVis 2017 reviews.

During VIS 2017, some authors of this paper also attended the *Workshop on Immersive Analytics: Exploring Future Interaction and Visualization Technologies for Data Analytics* (<http://immersiveanalytics.net/>). We appreciate the overwhelming interest and enthusiasm shown by the attendees in the topic of visualization in virtual environments. We also noticed that many questions raised during the workshop could be rephrased as an optimization problem about the balance of the three key factors, and be addressed from the angle of cost-benefit analysis. This confirms the applicability of this work. We therefore attempted our answers to 13 questions (out of 16) in the list that can be found at <https://goo.gl/d5pbRG>. As part of our revision, we added a new section (Section 8) to describe this exercise, and added a new Appendix C with all 13 answers.

When the original paper was converted to the EuroVis format, the main body took up 12 pages. We therefore significantly shortened two evidence sections (Sections 5 and 6), while moving the full texts of these two sections to Appendices A and B respectively. This allowed us to reduce the main body of the paper to about 10.3 pages. With the addition of Section 8, we managed to use 11 pages for the main body.

We are aware that the recommendation from EuroVis is to use 10 pages for the main body of the paper though this is not a strict limit. We think that the broad coverage of the discourse in this paper perhaps justifies the use of one more page than the recommendation. We hope that this will be OK.

Thank you very much for your consideration.

Yours faithfully

Authors (anonymous for the review process)

---

### Authors Feedback to the SciVis Reviews

**1. Summary Review:** The consensus among the reviewers was that this paper lacked practical knowledge that readers could apply and that it attempts to cover too many areas.

**Action:** We think that the new additions of Section 8 and Appendix C will address this issue raised. We are aware that main readers would like to see a set of initiate guidelines for designing better applications. The cost-benefit analysis based on information indicates that many design problems that readers are facing are optimization problems about a balancing act with the three key factors. Our answer to Q11 in Section 8 is a demonstration for analyzing the three factors.

**2. Summary Review:** However, the reviewers did like the general idea. Two reviewers were concerned about the reliance on reference [19] and suggested that the authors summarize more of that particular previous work within the text of this paper.

**Clarification and Action:** We appreciate that many readers in VIS and VR have limited knowledge about information theory, and it may take some time for the mathematical formulation in [19] to become comprehensible to many. This paper provides another opportunity to connect the theory with applications. We believe that the more such effort is made and the more VIS researchers are doing so, the more comprehensible the original mathematical formulation will become. To alleviate the difficulties in thinking about the non-mathematical form of the cost-benefit metric in [1], we added a few more principles that can be derived from this metric in Section 4 (under the Heading of Cost-benefit Analysis)

**3. R4:** Why is it true that "any increase of immersion and presence will most likely result in an increase of the size and complexity of alphabet V?"

**Clarification:** This relates to the fundamental approach of information theory, which considers a set of all possible scenarios rather a particular scenario. In VIS, we often discuss how to visualize a dataset (i.e., a letter) in order to make some observations. With information theory, we need to consider all possible datasets (i.e., an alphabet) that may be visualized and what observations that may be made with all such possibility. In principle, the latter way of thinking allows us to anticipate usefulness of a visualization method by considering all possible datasets rather than just one in front of us now. Back to the above question, when we introduce more immersion and presence, we usually introduce more variables from the users' point of view (e.g., more pixels, more depth resolution, more sound, more means to interact, ...), so the users will expect more variations in what they can see and hear, etc. All these possible variations are letters in alphabet V. This is a more powerful way of thinking about visualization. As discussed in (2), most of us can think in this way, and it just takes some time to get accustomed to.

**4. R4:** I would like to see citations to support your assertion in Sec 5 Attention paragraph: "These additional movements also incur additional requirements for information retention. ..."

**Clarification:** It is relatively obvious. When one turns one head to pay attention to a different part of a very large display screen, the part of the screen that has disappeared from the field of view can only be known to the viewer through some information retention.

**5. R1:** I'd rather see a more focused paper on visual analysis tasks, which are quite distinct from the goals of simulation training and educational applications. ... It is currently too broad in its focus.

**R2:** The paper is interesting but I think it tries to tackle too broad an area

**Clarification:** We disagree with these comments. We believe that addressing a broad set of applications in VEs using the same theory allows us to see the balancing act of the three key components in different scenarios. While a focused discussion on one type of applications is useful, it has the risk of leading readers to a biased conclusion, e.g., VR has worked in some training, it must also works in any training, and likely works in visual analytics. We think that this paper gives a holistic and theoretic treatment that has not been seen previously in either VIS or VR.

**6. R2:** The authors state that "visualization tasks are expected to be the same for a gigapixel display and a few megapixel displays." I disagree with this statement.

**Clarification:** This is about comparing two different types of displays under the same conditions. Having the same tasks facilitates a fair and objective comparison. The reviewer may have had the experience of using two types of displays (e.g., A and B) for different tasks (e.g., X and Y) based on some reasoning of the relative merits. This above statement only implies that let us compare A with (X, Y) against B with (X, Y).

**7. R2:** The authors state that "since VEs normally cost more than an everyday visualization environment, what is the benefit that would justify the extra cost? - What is an everyday visualization environment? a laptop? a whiteboard? a big TV? At the low end a VE could cost roughly the same as an everyday visualization environment."

**Clarification and Action:** We are aware and agree that the price of some types of VE devices are coming down, while many VEs environments are still in the form of large infrastructures, that is why we use the adverb "normally". In general, since many low-cost VE devices still require the support of a desktop computer, and those VE displays are usually bought in addition to a conventional display. So we think that our statement is correct. It is also important that our analysis considers both economic cost and cognitive cost. Nevertheless we have added a statement in the conclusion to echo the cost reduction.

**8. R3:** While the theory/model from 19 was used for VE, it would have nice to see some benefit/cost ratio computed for few use-cases.

This question was raised by the TVCG reviewers of [19] where the cost-benefit metric was proposed. Here we reuse the answer below. Since then some progress has been made, slowly, with a paper in IEEE VAST 2016 on estimating some quantitative values and another paper in EuroVis 2017 on obtaining measurements using empirical studies. We believe that such estimation and measurement works will follow in the future.

A credible **information-theoretic measurement experiment** needs at least two alphabets, each with a number of letters. The input alphabet needs to have more letters than the output alphabet and much more if it involves a numerical primitive variable(s). For each letter in both alphabets, we need to establish its probability. Hence each letter needs to be sampled for a number of times to obtain a statistically significant probability value. This can be done relatively easily for a machine-centric process through the monitoring of the input and output streams. However, it will be time-consuming to do this in a human-centric experiment. For a very simple study (may be too simple to be informative), for example, if the input alphabet  $X$  is defined by three variables (e.g., a 3-bar barchart), and each variable has 10 valid values, we have 1000 letters in the input alphabet. If the output is a simple decision with 5 options, we have 5 letters in the output alphabet  $Y$ . We also need to measure the distributions of the alphabets  $X'_m$  and  $X'_h$  from the machine-centric and human-centric reverse functions. At least  $X'_h$  has to be measured by an empirical study. Collecting the probability distributions for 1000 letters meant 1000 variables in an empirical study. The first author has designed or led a number of empirical studies (some with help from psychologists). A typical controlled laboratory study handles about 1-3 variables, and 2-4 values per variable, i.e., 2-12 letters. Note that  $12 \ll 1000$ . Hence, "**information-theoretic measurement experiment**" poses the second challenge due to the size of the empirical studies required. In general, the technology for measuring the humans' thinking and analytic processes is in its infant stage. However this does not mean that this can never be achieved.

Anyone familiar with thermodynamics would also know that an entropy quality in thermodynamics is not usually obtained through a measurement based on its statistical molecular behaviours within a system. It is usually measured through related components in the first and second laws. It took more than 1000 years for scientists to discover various ways of measuring temperature indirectly, e.g., using volume and pressure, e.g., from Claudius Galenus, to Gabriel Fahrenheit to William Lord Kelvin. This challenge also partly cost Ludwig Boltzmann's life. Optimistically, if there is more fundamental research in the field visualization, indirect measurements of information-theoretic qualities in human-centric processes will eventually be discovered.

## 9. R1, R2, R3, R4: All minor revisions and references.

**Action:** Done. Thank you.

---

## The Original Text of SciVis 2017 Reviews

Dear (Anonymous Author)

We regret to inform you that we are unable to accept your SciVis 2017 Papers submission:

132 - Cost-benefit Analysis of Visualization in Virtual Environments

The reviews are included below. This year, IEEE SciVis had 120 submissions and we conditionally accepted 27, for a provisional acceptance rate of 22%.

There were many factors considered in evaluating the reviews. Although numerical scores are important, we also read reviewers' comments and discussion closely to understand their reasons for the scores. We arrived at the final decision by balancing all of these different points of view.

Many of the submissions that were not accepted present interesting work and ideas. We hope you will find the reviewers' comments informative, especially if you revise your paper for submission to next year's conference, TVCG, or elsewhere.

We particularly encourage this where the ideas contained in submissions were positively received by reviewers but the revisions required were deemed to be beyond the scope of the conference review cycle. If you address the issues raised and subsequently submit to TVCG, please make reference to the SciVis 2017 Papers submission and include a description of how you addressed the SciVis 2017 Papers reviewers' comments.

Please also consider submitting work that was received positively to the IEEE VIS 2017 Posters program, due on June 16. This will enable you to still present your work to the VIS audience and get further feedback on your ideas. For more information, see <http://ieevis.org/year/2017/info/call-participation/posters>

We thank you for submitting your paper to SciVis 2017 Papers. We wish you the best in your endeavors and still hope to see you at the conference. Please check online for updates on this year's program - <http://www.ieevis.org/>

---

----- Submission 132, Review 4 -----

Title: Cost-benefit Analysis of Visualization in Virtual Environments

Reviewer: primary

Paper type

Theory / Model

Expertise

2 (Knowledgeable)

Overall Rating

<b>3 - Possible Accept</b><br/> The paper is not acceptable in its current state, but might be made acceptable with significant revisions within the conference review cycle.<br/>If the specified revisions are addressed fully and effectively I may be able to return a score of '4 - Accept'.

Supplemental Materials

Not applicable (no supplemental materials were submitted with the paper)

Justification

Authors give theoretical discussion of cost-benefit model of first author (previous work) applied to visualization in various forms of virtual environment. The theory discussion is challenging to read and would benefit from better connection to practical applications (material in Section 6, but these cover only two forms of VEs). I think this discussion is thus incomplete to give the model. Perhaps this can be fixed within a review period, but it will be hard to complete and even harder to check in the time available. So while the ideas are interesting, I don't see them as usable in their current form for most people. So my score is in the middle.

The Review

I have questions about detailed conclusions and concerns about the paper organization that I think would make it more complete and make it more useful to readers. But it really needs to fill in the holes in examples that are not included for all types of VEs. The evidence from cognitive science section is not well-integrated with the rest of the discussion. And this material is likely unfamiliar to most VIS attendees.

Why is it true that "any increase of immersion and presence will most likely result in an increase of the size and complexity of alphabet V?" Are there more states possible because the VE user has presence? I do not understand this conclusion (section 4, Alphabets and Letters).

I would like to see citations to support your assertion in Sec 5 Attention paragraph: "These additional movements also incur additional requirements for information retention. Hence, there is a high cognitive load for maintaining a certain level of awareness across the external information available." This disagrees with my understanding of spatial cues for memory (though this is not my expert area).

Regarding Fig.2, why are process 3 and 6 never used?

I found myself wanting more practical examples all through Section 4. I think at least some references forward from Section 4 to Section 6 would help, though I would prefer integrating by application first and then step through the model. This would need major rewriting, though. I am not finding much help in Section 6 for how I can use this, either.

In 4.1, bullet list

#2: much more -> many more

#4: an phenomenon -> a phenomenon

I think you have one line of text on page 10, which is technically not allowed. Minor to fix, I hope.

Summary Rating

2 (<b>Reject</b><br/> The paper is not ready for publication in SciVis / TVCG.<br/>The work may have some value but the paper requires major revisions or additional work that are beyond the scope of the conference review cycle to meet the quality standard. Without this I am not going to be able to return a score of '4 - Accept'.)

## The Summary Review

The consensus among the reviewers was that this paper lacked practical knowledge that readers could apply and that it attempts to cover too many areas. Fixing these are requirements for acceptance, and this was not seen as something that could be addressed in the review cycle. On this basis, the recommendation is to reject it for VIS 2017.

However, the reviewers did like the general idea. Two reviewers were concerned about the reliance on reference [19] and suggested that the authors summarize more of that particular previous work within the text of this paper.

Second round comments (public)

(blank)

Second round supplementary materials check

(blank)

Second round supplementary materials comments

(blank)

----- Submission 132, Review 1 -----

Title: Cost-benefit Analysis of Visualization in Virtual Environments

Reviewer: external

Paper type

Theory / Model

Expertise

2 (Knowledgeable)

Overall Rating

<b>2 - Reject</b><br/>The paper is not ready for publication in SciVis / TVCG.<br/>The work may have some value but the paper requires major revisions or additional work that are beyond the scope of the conference review cycle to meet the quality standard. Without this I am not going to be able to return a score of '4 - Accept'.

Supplemental Materials

Not applicable (no supplemental materials were submitted with the paper)

Justification

An ambitious paper that analyzes the costs and benefit associated with virtual environments in a broad range of applications (visual analytics, education, training/simulation). However, the information-theoretic analysis sometimes leads to obvious conclusions (e.g., when analyzing the cost-benefits of simulation/training applications). At other times, important factors (e.g., the benefits of embodied cognition and spatial memory) are not included or not clearly illustrated. The generality and broad focus of the paper seems to hurt the depth/validity of the analysis.

The Review

This paper analyzes the benefits and costs of using virtual environments (VE) in visualization. The authors adopt an information theory framework to understand the merits of immersion. Using this framework as a lens, they analyze previously-reported uses of VEs in the vis community along with relevant cognitive science findings.

This paper sheds a light on an important question, namely under what circumstances do immersive environments benefit visualizations to justify their cost? The paper is quite ambitious in its scope; the analysis covers a wide range of VE systems (virtual reality, large displays, domes) and a variety of use cases (education, simulation-based training, and visual analytics). The information theory framework provides interesting constructs (e.g., the notion alphabet compression) that allow theoretic comparison between a traditional and VE-based vis, given the same dataset and task. In some instances, this comparison seems to contribute new insights. For instance, when the authors justify the use of larger displays based on the degree of variation within the dataset and the need to revisit parts of the data during the analysis.

That said, the information-theoretic analysis seems a bit of an awkward fit and not quite as informative when looking at educational and simulation applications. The results here were hardly surprising: the more realistic the simulation is, the more likely it is to be successful in inducing training (if it's not known in advance which sensory information is relevant to training). When we

know that certain sensory information is not important in the original task, those can be safely removed from the simulation to reduce cost. These are self-evident results and wouldn't need information theory to justify, but yet constitute a big chunk of the paper. It is understandable that the authors want to demonstrate the broader utility of their framework, but I feel this wider emphasis is a bit distracting and serves only to dilute the substance of the paper.

I'd rather see a more focused paper on visual analysis tasks, which are quite distinct from the goals of simulation training and educational applications. A particularly interesting use case the authors seem to have overlooked is data monitoring and situation awareness, where big / immersive displays proliferate (e.g., in power plant operation and emergency response centers, etc...). How does the information theory framework account for the presumably large benefit here (given the large adoption rate despite the cost)?

I also urge the authors to consider other important factors in their analysis, including spatial memory and embodied cognition. The literature has shown these play an important role in improving performance for big displays, and hence should be thought of more than 'distortions'. How does the framework account for those benefits? I encourage the authors to explicitly include those (and possibly other related) factors in their framework, albeit at the expense generality, or at the very least surface them in their analysis. Another important use case the authors might want to include is collaboration; this is often cited as an important reason for adopting large multi-user VEs.

I also disagree with the authors that there have not been use-cases that demonstrate benefits for VEs in more analytical scenarios (or abstractions of thereof); there are in fact few studies that could provide some evidence here:

Liu et al. Effects of display size and navigation type on a classification task. In CHI'14

Reda et al. Effects of Display Size and Resolution on User Behavior and Insight Acquisition in Visual Exploration. In CHI'15

It would be quite interesting to see if the information theory perspective can provide an analysis of those as well.

Overall, while I think this paper is ambitious, it is currently too broad in its focus. When it comes to scientific and visual analysis tasks, the comparison between VEs and desktop-based visualizations is done at a very high-level that it misses (or at least doesn't make clear) important differences (such as spatial memory, embodied cognition, the ability to spatially organize information with large displays). I urge the authors to more explicitly discuss those factors clearly. I also suggest considering other important use cases for large VEs, such as collaborative analysis and monitoring/situation awareness. Those are more relevant to the vis community and, I suspect, are a more natural fit for an information-theory analysis.

----- Submission 132, Review 2 -----

Title: Cost-benefit Analysis of Visualization in Virtual Environments

Reviewer: secondary

Paper type

Theory / Model

Expertise

2 (Knowledgeable)

Overall Rating

<b>3 - Possible Accept</b><br/> The paper is not acceptable in its current state, but might be made acceptable with significant revisions within the conference review cycle.<br/>If the specified revisions are addressed fully and effectively I may be able to return a score of '4 - Accept'.

Supplemental Materials

Not applicable (no supplemental materials were submitted with the paper)

Justification

The paper is interesting but I think it tries to tackle too broad an area, in particular with the inclusion of training, and could instead use that space to better define some of their terminology, refine their text on user interaction, add more on collaboration, and give more examples within a more limited scope.

The Review

I think there is good work here, and parts of the paper are very interesting, but as someone who has worked in virtual environments and visualization for 25 years the paper is hard to follow at points. I need more background on the theoretical side of things and better definitions of some of the terminology used in the paper. I also have a hard time seeing right now how I would make use of

this in my work, given how general it is. I think the potential is definitely there, but I'd like the authors to help bring me into their world more, and focus the work more so the applications of it are more obvious.

The training area seems to have a very different profile from the others and, personally, seems like it belongs in a different paper, and if so, that space could be used to improve the discussion of the other areas. Training seems like a very different beast with a much greater focus on recreation of real world interaction as opposed to using interaction techniques that are more appropriate for the visualization / analysis / education work at hand. Even the paper itself seems to have different views on this area. The paper says that "The primary reason for using VE-based training is the lack of access to the required reality " and then the next sentence says the opposite. I very much disagree with the first statement, but agree with the next ones.

I think that maybe the paper focuses too much presence at the expense of natural interaction with the virtual worlds or visualizations. Virtual Environments with a variety of tracking allows users to interact with these spaces in various ways and that is critically important. The motor coordinate paragraph starts to go off in a variety of directions at the end of the paper where interaction was hardly discussed before - e.g. does the blacksmith reference belong here? Natural interaction using our bodies is crucial in VEs , and taking the limitations of the human body into account when designing physical and virtual worlds is critical, but interaction doesn't seem to get enough attention here, in my opinion, given the wide variety of devices available and ways to interact with abstract information in (perhaps) limitless ways.

The paper starts going really deep in section 4 without bringing the more general VE / visualization reader (like myself) along. It would help to have better discussion of alphabet compression, decision alphabet, reconstructed alphabet, shannon entropy.

I think that section 7 (4 levels of visualization) should come earlier.

I'm surprised there was no discussion of ensembles in 4.3

The authors state that "visualization tasks are expected to be the same for a gigapixel display and a few megapixel displays. " I disagree with this statement. I also disagree with "The user's prior knowledge about the dataset and its visualization usually reduces the cost-benefit of using a gigapixel display. " I'd like to read what experiences and references the authors have for these statements as they are different from my experiences.

The authors state that "since VEs normally cost more than an everyday visualization environment, what is the benefit that would justify the extra cost? - What is an everyday visualization environment? a laptop? a whiteboard? a big TV? At the low end a VE could cost roughly the same as an everyday' visualization environment. Perhaps it wouldn't have as many capabilities as a more (expensive / powerful) one but I don't think this general statement is true, so I'd like more details on what the authors are thinking here.

The authors also state that "The more cognitive resources are devoted to the attention for retrieving external information, the less cognitive resources are available for the attention to internal events (e.g., analytical reasoning and decision making). " I agree that demand has to be carefully managed, but if you can't see all the information on the screen at one time then you have to resort to recall, as discussed a bit further down in the paper. This brings up the larger issue of organization, and perhaps having too large a scope to the paper, as I think given the wide scope of the paper its hard to put content into (what I consider) a good order as there are so many different possible orderings here.

I think there are at least two papers here, and I'd like to read those papers but I don't think they are written for this audience right now.

----- Submission 132, Review 3 -----

Title: Cost-benefit Analysis of Visualization in Virtual Environments

Reviewer: external

Paper type

(blank)

Expertise

3 (Expert)

Overall Rating

<b>3.5 - Between Possible Accept and Accept</b><br/>

Supplemental Materials

Not applicable (no supplemental materials were submitted with the paper)

Justification

The paper presents an interesting work on the evaluation of different VR systems (VR/AR) using a cost-benefit analysis that provides insight on why some visualization benefit more from VR than others. The strength of this paper is providing a model/theory that could be used to evaluation variations of VR application. The weakness of the paper is a lack of quantitative information on the evaluation.

#### The Review

The paper "Cost-benefit Analysis of Visualization in Virtual Environments" intends to provide a theory/model to evaluate which visualization application will benefit most from the use of Virtual Environments. The topic is very interesting as this is one of the most frequently asked questions by researchers, and end-users.

When I read the title of the paper, I was expecting to see some table with numbers for each kind of VR applications that will be computed based on some model/theory. The paper did present a model and used that for the discussions in the paper, however, it lacks some real numbers. Since alphabet compression was seldom used, it would have been nice to include a short paragraph on it as well in the paper to make it self-contained. Also, it was noticeable that this paper referred to reference [19] many times throughout the paper.

Overall the paper is easy to follow once you also read the paper [19]. Without reading that reference, it would be harder for readers to get the full grasp of the concepts presented in this paper. It would have been nice to introduce some of these concepts in this paper as well as mentioned earlier.

While the paper is interesting and useful, I felt that somehow the paper loses the attention on cost-benefit analysis in later sections, but the paper covers different kinds of VR applications well, very well defines the immersion and presence and uses that in the discussions, and provides some concrete examples.

#### Revision Required

=====

1. In Section 1 "Introduction," suchcost should be such cost (and no italics).
2. Perhaps the authors could have added a reference to Shannon Entropy (from Information Theory) for readers who are unfamiliar with the topic?
3. While the theory/model from 19 was used for VE, it would have nice to see some benefit/cost ratio computed for few use-cases.
